# Supplementary material for: Target Aggregate Data Adjustment Method for Transportability Analysis Utilizing Summary-Level Data from the Target Population
Source: arXiv:2412.12335 source file (2025-07-07)
Supplement: Supplementary file 1 [file TADA_Supplementary_v0_1.pdf]

# SUPPLEMENTARY MATERIAL

## Target Aggregate Data Adjustment Method for Transportability Analysis Utilizing Summary-Level Data from the Target Population

Yichen Yan<sup>1,2</sup>, Quang Vuong<sup>2</sup>, Rebecca K Metcalfe<sup>2,3</sup>, Tianyu Guan<sup>4</sup>,  
Haolun Shi<sup>1</sup>, Jay JH Park<sup>2,5\*</sup>

<sup>1</sup>Department of Statistics and Actuarial Science

Simon Fraser University

BC, Canada

<sup>2</sup>Core Clinical Sciences

BC, Canada

<sup>3</sup>Centre for Advancing Health Outcomes

University of British Columbia

BC, Canada

<sup>4</sup>Department of Mathematics and Statistics

York University

ON, Canada

<sup>5</sup>Department of Health Research Methodology, Evidence, and Impact

McMaster University

ON, Canada

*\*email:* parkj136@mcmaster.ca

### S.1 Overview of Existing Transportability Analysis Methods for Aggregate Data

The existing empirical work on transportability analysis methods that can handle aggregate target data has largely focused on entropy balancing. [1, 2, 3, 4]. Entropy balancing was first proposed by Hainmueller [2] to estimate the average treatment effect on the treated

(ATT). It constructs the weights for the control units as the solution to an optimization problem. Entropy balancing adjusts the weighted control group's covariate averages to align with those of the treated group. Concurrently, to make the weight distribution as uniform as possible, the optimization goal reduces the dispersion metric, which is essentially the inverse of entropy. The optimization problem of entropy balancing in Hainmueller can be formulated as follows:

$$\begin{aligned} & \min_{w \geq 0} \quad \sum_{i \in S_0} w_i \log w_i \\ & \text{subject to} \quad \frac{1}{n_s} \sum_{i \in S_0} w_i X_i = \frac{1}{|S_1|} \sum_{i \in S_1} X_i, \quad \sum_{i \in S_0} w_i = n_s. \end{aligned}$$

Motivated by this framework, Josey et al. [3] and Lee et al. [7] adapted the entropy balancing approach for generalizing and transporting ATE estimation from an RCT to a given target population, respectively. Chen et al. [1] noted the equivalence of entropy balancing and exponential tilting adjustment [10] in the RCT setting, where these two methods share the same balancing constraints. As a follow-up, Josey and colleagues published further work on methods that can handle transporting observational data and established the double robustness properties of the weighting estimators [4]. They proposed a two-step method to mitigate covariate imbalance or confounding between the treatment and control groups in observational studies. In the first step, they solved the following problem to get  $\{\hat{q}_i\}$ :

$$\begin{aligned} & \min_{q \geq 0} \quad \sum_{i \in S} q_i \log q_i \\ & \text{subject to} \quad \frac{1}{n_S} \sum_{i \in S} q_i h_k(X_i) = \bar{h}_{k, \mathcal{T}}, \quad k = 0, \dots, K_h, \end{aligned}$$

and then adjusted for the treatment-control imbalance by solving the following as the second step:

$$\begin{aligned} & \min_{w \geq 0} \quad \sum_{i \in S} w_i \log \left( \frac{w_i}{\hat{q}_i} \right) \\ & \text{subject to} \quad \frac{1}{n_S} \sum_{i \in S_1} w_i h_k(X_i) = \frac{1}{n_S} \sum_{i \in S} \hat{q}_i h_k(X_i), \quad k = 0, \dots, K_h \\ & \quad \frac{1}{n_S} \sum_{i \in S_0} w_i h_k(X_i) = \frac{1}{n_S} \sum_{i \in S} \hat{q}_i h_k(X_i), \quad k = 0, \dots, K_h, \end{aligned}$$

where the constraints calibrate the treated and control groups to the same weighted trial sample. This approach is also available for transporting treatment effects in data-fusion cases. However, it requires IPD for both the trial population and target sample in such scenario [4].

Chen et al. retained the entropy balancing design in Josey et al. and added further balancing requirements between the treated and control groups in the source sample to further enhance the theoretical capacity [1]. This approach applied an additional set of functions  $\{g_k, k = 1, \dots, K_g\}$  as following:

$$\begin{aligned} & \min_{w \succeq 0} \quad \sum_{i \in S} w_i \log w_i \\ \text{subject to} \quad & \frac{1}{n_s} \sum_{i \in S_1} w_i h_k(X_i) = \bar{h}_{k,T}, \quad k = 0, \dots, K_h \\ & \frac{1}{n_s} \sum_{i \in S_0} w_i h_k(X_i) = \bar{h}_{k,T}, \quad k = 0, \dots, K_h \\ & \frac{1}{n_s} \sum_{i \in S_1} w_i g_k(X_i) = \frac{1}{n_s} \sum_{i \in S_0} w_i g_k(X_i), \quad k = 1, \dots, K_g. \end{aligned}$$

The enhanced approach offers better versatility, enabling the weights to rely on  $\{g_k\}$ . This set of covariate functions is significantly broader than  $\{h_k\}$ , providing a more comprehensive approach to weighting.

To account for the possible violation of the PH assumption during transporting survival outcomes, Lee et al. [6] extended the augmented calibration weighting (ACW) method [8] by incorporating the hazard regression model based on linear splines (HARE) [5], which does not rely on the PH assumption. The ACW method combines both calibration weighting and outcome regression under the PH assumption to estimate treatment effects in the target population, with the properties of double robustness and local efficiency. The HARE model is expressed as:

$$\log \lambda_a^H(t \mid X_i) = \sum_{k=1}^p \beta_{ak}^H B_k(t \mid X_i),$$

where  $B_k(t \mid X_i)$  are spline basis functions that allow for non-linear relationships between time and covariates. The inclusion of the HARE model significantly enhances the robustness of the ACW estimator, enabling it to handle complex survival data scenarios such as delayed treatment effects or crossing survival curves. The simulation results show that the extended

method ensures more reliable and accurate treatment effect estimates across diverse target populations.

Despite its popularity, entropy balancing approaches for transportability suffer from some notable drawbacks. The complicated statistical structure directly increases the sensitivity of assumptions [1, 3, 4, 6]. It can also have a slow convergence rate since the probability that a feasible weighting solution exists decreases in small samples [3]. An alternative is to incorporate the MoM balancing weights into the TMLE framework and set up a targeted maximum likelihood-type estimator given limited target data [3]. Although the holistic structure of the EB method allows it to achieve one-step balancing across complex constraints, this simultaneously weakens its clinical interpretability, which is crucial in practice [9, 11]. The intricate optimization process underlying EB can obscure the clinical rationale behind weighting adjustments, making the method less accessible for practitioners who seek clear, step-by-step insight into the adjustment process.

## References

- [1] Rui Chen, Guanhua Chen, and Menggang Yu. Entropy balancing for causal generalization with target sample summary information. *Biometrics*, 79(4):3179–3190, 2023.
- [2] Jens Hainmueller. Entropy balancing for causal effects: A multivariate reweighting method to produce balanced samples in observational studies. *Political Analysis*, 20(1):25–46, 2012.
- [3] Kevin P Josey, Seth A Berkowitz, Debashis Ghosh, and Sridharan Raghavan. Transporting experimental results with entropy balancing. *Statistics in Medicine*, 40(19):4310–4326, 2021.
- [4] Kevin P Josey, Fan Yang, Debashis Ghosh, and Sridharan Raghavan. A calibration approach to transportability and data-fusion with observational data. *Statistics in Medicine*, 41(23):4511–4531, 2022.

- [5] Charles Kooperberg, Charles J Stone, and Young K Truong. Hazard regression. *Journal of the American Statistical Association*, 90(429):78–94, 1995.
- [6] Dasom Lee, Chenyin Gao, Sujit Ghosh, and Shu Yang. Transporting survival of an hiv clinical trial to the external target populations. *Journal of Biopharmaceutical Statistics*, pages 1–22, 2024.
- [7] Dasom Lee, Shu Yang, Lin Dong, Xiaofei Wang, Donglin Zeng, and Jianwen Cai. Improving trial generalizability using observational studies. *Biometrics*, 79(2):1213–1225, 2023.
- [8] Dasom Lee, Shu Yang, and Xiaofei Wang. Doubly robust estimators for generalizing treatment effects on survival outcomes from randomized controlled trials to a target population. *Journal of Causal Inference*, 10(1):415–440, 2022.
- [9] Benjamin Lu, Eli Ben-Michael, Avi Feller, and Luke Miratrix. Is it who you are or where you are? accounting for compositional differences in cross-site treatment effect variation. *Journal of Educational and Behavioral Statistics*, 48(4):420–453, 2023.
- [10] James E Signorovitch, Eric Q Wu, Andrew P Yu, Charles M Gerrits, Evan Kantor, Yanjun Bao, Shiraz R Gupta, and Parvez M Mulani. Comparative effectiveness without head-to-head trials: a method for matching-adjusted indirect comparisons applied to psoriasis treatment with adalimumab or etanercept. *Pharmacoeconomics*, 28:935–945, 2010.
- [11] Caroline M Vass, Marco Boeri, Christine Poulos, and Alex J Turner. Matching and weighting in stated preferences for health care. *Journal of Choice Modelling*, 44:100367, 2022.
